# Supplementary material for: TEASER: Fast and Certifiable Point Cloud Registration
Source: arXiv:2001.07715 source file (2020-10-17)
Supplement: Supplementary file 1 [file appendix-scalarTLSthm.tex]

%!TEX root = main.tex

\subsection{Proof of~\prettyref{thm:scalarTLS}}
\label{sec:proof:scalarTLS}

\grayout{
\LC{still working on it}
Let us first prove that $\hats$ belongs to the set of optimal solutions of~\eqref{eq:consensusMax}. 
For this purpose, we first rewrite the consensus maximization problem equivalently as:
\beq
\label{eq:consensusMax_d}
(z^\star, \calS^\star) = \argmin_z \sumAllPoints 
\calI\left( \frac{(z - s_k)}{\alpha_k^2} > \barcsq \right) \cdot \barcsq
\eeq 
where we minimize the set of outliers rather than maximizing the inliers, and 
we multiplied the cost by a constant $\barcsq$. Let us call the objective in~\eqref{eq:consensusMax_d} $d(z)$ and the corresponding optimal value $d^\star$ (attained at some $z^\star$). We note that:
\bea
d^\star = (K - |\calS^\star|) \barcsq
\eea
where $\calS^\star$ is the consensus set (inliers) and $|\cdot|$ denotes the cardinality of a set.
Similarly, we rewrite~\eqref{eq:TLSscale} as:
\bea
\label{eq:LTSscale_f}
\hats = \argmin_{s} \sumAllIM 
\calI\left( \frac{(s - s_k)}{\alpha_k^2} \leq \barcsq \right) \cdot
\frac{  (  s-s_k )^2 }{  \alpha^2_k }   \\
+
\calI\left( \frac{(s - s_k)}{\alpha_k^2} > \barcsq \right) \cdot \barcsq
\eea
Let us call the objective in~\eqref{eq:LTSscale_f} $f(s)$ and the corresponding optimal value $f^\star$ (attained at $\hats$). For any choice of $s$: 
\bea
\label{eq:costIneq}
(K - |\calS^\star|) \barcsq = d^\star \leq d(\hats) \leq  f(\hats) = 
 f^\star \leq 
 \\
|\hat{\calS}|( \barcsq - \eps)
+
(K - |\hat{\calS}|) \barcsq = K \barcsq  - |\hat{\calS}| \eps
\eea
since $f(s)$ has additional positive terms.

% \bea
% (K - |\calS^\star|) \barcsq \leq K \barcsq  - |\hat{\calS}| \eps \iff\\
% |\calS^\star| \barcsq \geq |\hat{\calS}| \eps
% \eea

\bea
(K - |\hat{\calS}|) \barcsq \leq f^\star \leq \\
|\calS^\star|( \barcsq - \eps)
+
(K - |\calS^\star|) \barcsq = K \barcsq  - |\calS^\star| \eps \iff\\
|\hat{\calS}| \barcsq \geq |\calS^\star| \eps
\eea

\bea
(K - |\calS^\star|) \barcsq \leq (K - |\hat{\calS}|) \barcsq \iff\\
|\calS^\star| \geq |\hat{\calS}| 
\eea

Assume now by contradiction that $\hats$ is not an optimal solution to~\eqref{eq:consensusMax_d} and call $\hat{\calS}$ the consensus set of $\hats$, i.e.,:
\bea
\hat{\calS} = \setdef{ k = 1,\ldots,K }{  \frac{(\hats - s_k)}{\alpha_k^2} \leq \barcsq }
\eea
Since the optimal consensus set~\eqref{eq:consensusMax_d} is assumed to be unique, the suboptimality of $\hats$ implies that $| \hat{\calS} | < |\calS^\star|$ (this can be easily seen from~\eqref{eq:consensusMax} where the objective simply counts the number of inliers).
However, using~\eqref{eq:costIneq}:
\bea
 d(z^\star) \leq d(\hats) \leq  f(\hats) %= f^\star.
\eea
% comparing 
% \bea
%  d(z^\star) \leq d(\hats) \leq  f(\hats) = f^\star.
% \eea
Now recalling that $d(z^\star) = K - |\calS^\star| \barcsq$ and 
$d(\hats) = K - |\hat{\calS}| \barcsq$:
%, and using~\eqref{eq:costIneq}:
% this implies:
% \bea
%  d(z^\star) \leq d(\hats) \leq  f(\hats) = f^\star.
% \eea
\bea
 K - |\calS^\star| \barcsq \leq K - |\hat{\calS}| \barcsq \iff\
|\calS^\star| \geq |\hat{\calS}|
\eea
leading to contradiction.
}
