# Supplementary material for: TEASER: Fast and Certifiable Point Cloud Registration
Source: arXiv:2001.07715 source file (2020-10-17)
Supplement: Supplementary file 2 [file appendix-scaleBounds.tex]

%!TEX root = main.tex

\subsection{Computation of Scale Bounds}
\label{sec:appendix}

The two point clouds $\{\bm{b}_i\}_{i=1}^N$ and $\{\bm{e}_i\}_{i=1}^N$ are generated by (inliers):
\begin{align}
\bm{b}_i = s\bm{R}\bm{e}_i + \bm{t} + \bm{\epsilon}_i
\end{align}
where $s \in \mathbb{R}_{+}$ is the scale, $\bm{R}$ is the rotation matrix and $\bm{\epsilon} \sim \mathcal{N}(\bm{0},\bm{\Sigma})$ is the noise vector with zero mean and diagonal covariance matrix $\bm{\Sigma}=\text{diag}(\sigma^2,\sigma^2,\sigma^2)=\sigma^2 \bm{I}$. Now suppose we root point cloud $\{\bm{b}_i\}_{i=1}^N$ at $\bm{b}_r$ and point cloud $\{\bm{e}_i\}_{i=1}^N$ at $\bm{e}_r$ by subtracting $\bm{b}_r$ and $\bm{e}_r$ from all the points, and suppose both $\bm{b}_r$ and $\bm{e}_r$ are inliers:
\begin{align}
\tilde{\bm{b}}_i&=\bm{b}_i-\bm{b}_r \nonumber \\
&=s \bm{R} (\bm{e}_i - \bm{e}_r) + \bm{\epsilon}_i - \bm{\epsilon}_r \nonumber \\
&=s \bm{R} \tilde{\bm{e}}_i + \bm{\epsilon}_{ir} 
\end{align}
where $\bm{\epsilon}_{ir}=\bm{\epsilon}_i - \bm{\epsilon}_r \sim \mathcal{N}(\bm{0}, 2\bm{\Sigma})$. Using this expression, we can have an estimate of the scale $s$ using triangle inequality:
\begin{align}
&s_i = \frac{\Vert \tilde{\bm{b}}_i \Vert}{\Vert \tilde{\bm{e}}_i \Vert}= \frac{\Vert s \bm{R} \tilde{\bm{e}}_i + \bm{\epsilon}_{ir}  \Vert}{ \Vert \tilde{\bm{e}}_i \Vert } 
 \geq \frac{s\Vert \bm{R} \tilde{\bm{e}}_i  \Vert - \Vert \bm{\epsilon}_{ir}  \Vert}{\Vert \tilde{\bm{e}}_i \Vert} = s-\frac{\Vert \bm{\epsilon}_{ir}  \Vert }{\Vert \tilde{\bm{e}}_i \Vert} \nonumber \\
&s_i = \frac{\Vert \tilde{\bm{b}}_i \Vert}{\Vert \tilde{\bm{e}}_i \Vert}= \frac{\Vert s \bm{R} \tilde{\bm{e}}_i + \bm{\epsilon}_{ir}  \Vert}{ \Vert \tilde{\bm{e}}_i \Vert } 
 \leq \frac{s\Vert \bm{R} \tilde{\bm{e}}_i  \Vert + \Vert \bm{\epsilon}_{ir}  \Vert}{\Vert \tilde{\bm{e}}_i \Vert} = s+\frac{\Vert \bm{\epsilon}_{ir}  \Vert }{\Vert \tilde{\bm{e}}_i \Vert} \nonumber \\
&\Rightarrow s-\frac{\Vert \bm{\epsilon}_{ir}  \Vert }{\Vert \tilde{\bm{e}}_i \Vert} \leq s_i \leq s+\frac{\Vert \bm{\epsilon}_{ir}  \Vert }{\Vert \tilde{\bm{e}}_i \Vert}
\end{align}
where we can use the chi-square distribution to analyze the confidence level of $\frac{\Vert \bm{\epsilon}_{ir}  \Vert }{\Vert \tilde{\bm{e}}_i \Vert}$ starting from $\bm{\epsilon}_{ir} \sim \mathcal{N}(\bm{0}, 2 \sigma^2 \bm{I})$:
\begin{align}
\bm{\epsilon}_{ir} \sim \mathcal{N}(\bm{0}, 2 \sigma^2 \bm{I}) & \Rightarrow \frac{\bm{\epsilon}_{ir}}{\sqrt{2}\sigma} \sim \mathcal{N}(\bm{0}, \bm{I}) \nonumber \\
& \Rightarrow \frac{\Vert \bm{\epsilon}_{ir} \Vert^2}{2 \sigma^2} \sim \bm{\chi}^2(3) \nonumber \\
& \Rightarrow \mathbb{P} \left( \frac{\Vert \bm{\epsilon}_{ir} \Vert^2}{2 \sigma^2} < 11.35 \right) > 99\% \nonumber \\
& \Rightarrow \mathbb{P} \left( \frac{\Vert \bm{\epsilon}_{ir} \Vert^2}{\Vert \tilde{\bm{e}}_i \Vert^2} < \frac{22.7 \sigma^2}{\Vert \tilde{\bm{e}}_i \Vert^2} \right) > 99\% \nonumber 
\end{align}
Hence, we can bound $s_i$ as follows:
\begin{align}
\mathbb{P}\left( s-\frac{\sqrt{22.7} \sigma}{\Vert \tilde{\bm{e}}_i \Vert}  < s_i <  s+\frac{\sqrt{22.7} \sigma}{\Vert \tilde{\bm{e}}_i \Vert} \right) > 99\%
\end{align}
Alternatively, computing $s_i$ gives bounds for the true scale $s$:
\begin{align}
\mathbb{P}\left( s_i -\frac{\sqrt{22.7} \sigma}{\Vert \tilde{\bm{e}}_i \Vert}  < s <  s_i +\frac{\sqrt{22.7} \sigma}{\Vert \tilde{\bm{e}}_i \Vert} \right) > 99\%
\end{align}
Denote $c_i=\frac{\sqrt{22.7} \sigma}{\Vert \tilde{\bm{e}}_i \Vert}$, we design our optimization regarding $s$ as:
\begin{align}
s^*= \argmin_{s \in \mathbb{R}_{+}, \theta_i^2=1} \frac{1+\theta_i}{2} \left( s-s_i \right)^2 + \frac{1-\theta_i}{2} c_i^2
\end{align}
