# Supplementary material for: TEASER: Fast and Certifiable Point Cloud Registration
Source: arXiv:2001.07715 source file (2020-10-17)
Supplement: Supplementary file 3 [file appendix-maxConsensusAlgo.tex]

%!TEX root = main.tex

\subsection{Proof of~\prettyref{thm:maxConsensusAlgo}}
\label{sec:proof:maxConsensusAlgo}
