# Supplementary material for: TEASER: Fast and Certifiable Point Cloud Registration
Source: arXiv:2001.07715 source file (2020-10-17)
Supplement: Supplementary file 4 [file appendix-proofSufficientOptimalityCondition.tex]

%!TEX root = ../main.tex

\subsection{Proof of Theorem~\ref{thm:sufficientConditionGlobalOptimality}}
\label{sec:proofSufficientOptimalityCondition}
